# Supplementary material for: Distinct excitatory and inhibitory bump wandering in a stochastic neural field
Source: arXiv:2203.02438 source file (2022-03-04)
Supplement: Supplementary file 1 [file ex_supplement.tex]

% SIAM Supplemental File Template
\documentclass[final,supplement,onefignum,onetabnum]{siamart190516}

\input{ex_shared}

%% Use \myexternaldocument on Overleaf
% \myexternaldocument{ex_article}

% Optional PDF information
\ifpdf
\hypersetup{
  pdftitle={Supplementary Materials: Dynamics of Wandering Bumps in Two Population Stochastic Neural Field Networks},
  pdfauthor={H. Cihak, T. Eissa, and Z. Kilpatrick}
}
\fi

\begin{document}
\maketitle


\end{document}
